# Supplementary material for: Screen2Bench: From Screen Recordings to Faithful and Verifiable Computer-Use Benchmarks
Source: arXiv:2611.39246 source file (2026-11-29)
Supplement: Supplementary file 1 [file appendix.tex]

% Optional supplementary subsections. All content is intentionally blank.
\subsection{Assumptions}
\subsection{Analysis}
\subsection{Additional Results}
\subsection{Discussion}
